# Supplementary material for: Auto-Test: Learning Semantic-Domain Constraints for Unsupervised Error Detection in Tables
Source: arXiv:2504.10762 source file (2025-04-14)
Supplement: Supplementary file 1 [file Appendix-Multi-Outlier.tex]

\section{Extend to Report All Detected Errors in Online Prediciton Stage} 
\label{apx:multi-outlier}

\yeye{i have changed detection stage => online inference, Training => offline training, etc. (Figure 1), we can update in other places too}
The Detection Stage of \at can be naturally extended to report all detected errors in a test column. 
For a given column $C$, we first apply all \sdca in $R$ that are applicable to $C$ (i.e., \sdca whose pre-conditions evaluate as true on $C$) to get the errors predicted by each of them. 
Then, the set of reported errors in $C$ (i.e., $o(C,R)$) is simply set to the union of the predicted errors. 
The confidence of each reported error can be assigned as the highest confidence among all \sdca that detect it.

It is worth noting that all definitions, theorems, and proofs provided in the main paper extend seamlessly to this approach without modification.
% In this multiple-outlier extension, let $o(c, R)$ denote the set of outliers reported by $R$ on a column $c$. Note that in the single-outlier setting in our main paper, $o(c, R)$ is a single outlier (i.e., a single value), while in this extension $o(c, R)$ is a set of values.
% We consider a column $c$ as a FP if $o(c, R) \nsubseteq O(c)$, i.e., some non-outlier is returned.
% It is worth noting that all definitions, theorems and proofs developed in the main paper are applicable to the multiple-outlier setting as well, by simply replacing all occurrences of $o(c, R) \in O(c)$ (or $o(c, R) \notin O(c)$) with $o(c, R) \subseteq O(c)$ (or $o(c, R) \nsubseteq O(c)$).
% We consider a column $c$ as a FP if $o(c, R) \nsubseteq O(c)$, i.e., some non-outlier is returned.
% The FPR of set $R$ is defined as $fpr(R) = \frac{\left | \{c \in \mathcal{C} \,|\,  o(c, R) \nsubseteq O(c)\} \right |}{\left | \{ c \in \mathcal{C} \,|\, O(c) = \{\} \}\right |}$.
% To report multiple outliers for a column, in Detection Stage, we set the set of outliers detected by rule $r$ in a column $c$ to be all values in $c$ that falls in $r$'s constraint. Mathematically,  $o(c, \{r\}) = const(r) \cap c$. After deciding $o(c, \{r\})$ for every $r \in R$, $o(c, R)$ is simply the union of outliers reported by each rule. 
